# Supplementary material for: Microstructure-property prediction of a Ni-based superalloy: A combined phase-field and finite element modelling approach
Source: arXiv:2310.04885 ancillary file (2023-10-07)
Supplement: Supplementary file 1 [file Supplementary_CMS.pdf]

# Supplementary Material

## Multiscale study of microstructure evolution in Ni-Al alloys

Rupesh Chafle<sup>a,\*\*</sup>, Vishal Panwar<sup>a,\*\*</sup>, Somnath Bhowmick<sup>a</sup>, Kaushik Das<sup>b</sup>, Rajdip Mukherjee<sup>a,\*</sup>

<sup>a</sup>Department of Materials Science and Engineering, Indian Institute of Technology Kanpur, Kanpur 208016, India

<sup>b</sup>Department of Metallurgy and Materials Engineering, Indian Institute of Engineering Science and Technology Shibpur, Howrah 711103, India

### 1. Computing Elastic Constants by Density Functional Theory

#### 1.1. Computational details

Structural optimizations and elastic constant predictions are performed by using the density functional theory (DFT) based *ab initio* calculations, as implemented in the Quantum Espresso package [1]. The kinetic energy cut-off for the plane-wave basis set is taken to be 50 Ry. A  $10 \times 10 \times 10$  k-point mesh is used for Brillouin zone sampling during the self-consistent calculations to obtain the electronic ground state. Structural optimizations are carried out until the energy difference between two successive steps is less than  $10^{-4}$  Ry. Using the mcsqs code [2], quasi-random structures are generated based on a  $3 \times 3 \times 3$  face-centered cubic (non-primitive) super-cell, mimicking random distribution of Ni and Al atoms in the  $\gamma$  phase.

#### 1.2. Elastic Constants $C_{11}$ , $C_{12}$ and $C_{44}$

For calculating  $C_{11} - C_{12}$ , a cubic cell is deformed by a volume conserving orthorhombic strain [3],

$$\varepsilon = \begin{bmatrix} \delta & 0 & 0 \\ 0 & -\delta & 0 \\ 0 & 0 & \frac{\delta^2}{1-\delta^2} \end{bmatrix}. \quad (1)$$

The change of energy as a function of  $\delta$  is given by,

$$E(\delta) = E(0) + V(C_{11} - C_{12})\delta^2, \quad (2)$$

where  $V$  is the volume of the unit cell and  $E(0)$  is the energy at equilibrium volume ( $\delta = 0$ ). Value of  $\delta$  is varied from 0 to 0.04 in an interval of 0.01, and energy difference  $E(\delta) - E(0)$  is plotted as a function of  $\delta^2$  (see fig. S1). Value of  $C_{11} - C_{12}$  can be obtained by dividing the slope of the line (fig. S1) by the volume  $V$ ,

$$(C_{11} - C_{12}) = \frac{\text{slope of } [E(\delta) - E(0)] \text{ versus } \delta^2}{V}. \quad (3)$$

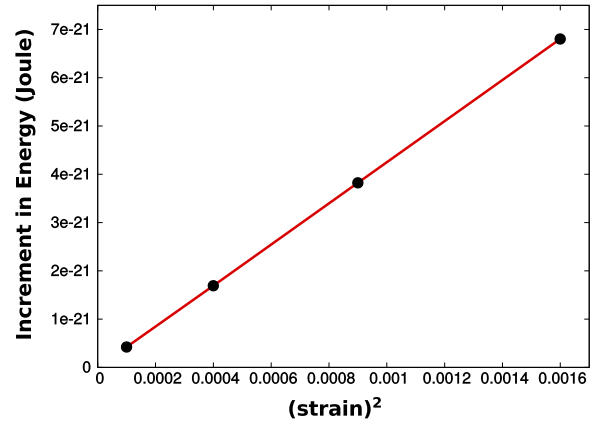

Figure S1: Change in energy versus  $\delta^2$  for a composition (Ni-0.12Al) of the  $\gamma$  phase at 1000 K, when a cubic cell is deformed by a volume conserving orthorhombic strain tensor.

Bulk modulus can be expressed in terms of  $C_{11}$  and  $C_{12}$  as,

$$B = \frac{(C_{11} + 2C_{12})}{3}. \quad (4)$$

A volumetric strain on the cubic cell (symmetry is conserved) is applied and energy is calculated as a function of volume. Bulk modulus is obtained by fitting the energy vs. volume data with some suitable equation of state, for example, the Murnaghan equation of state. Finally, the values of  $C_{11}$  and  $C_{12}$  can be obtained by solving equations 3 and 4.

For calculating  $C_{44}$ , a cubic cell is deformed by a volume conserving monoclinic strain [3],

$$\varepsilon = \begin{bmatrix} 0 & \frac{\delta}{2} & 0 \\ \frac{\delta}{2} & 0 & 0 \\ 0 & 0 & \frac{\delta^2}{4-\delta^2} \end{bmatrix}. \quad (5)$$

The change of energy as a function of  $\delta$  is given by,

$$E(\delta) = E(0) + V(C_{44})\delta^2, \quad (6)$$

where  $V$  is the volume of the unit cell and  $E(0)$  is the energy at equilibrium volume ( $\delta = 0$ ). Value of  $\delta$  is varied

\*Corresponding author

E-mail address: rajdipm@iitk.ac.in (R.Mukherjee)

\*\*These authors contributed equally to this work

Table S1: Calculated elastic constants for  $\gamma$  and  $\gamma'$  phases at 1000K.

| Phase     | %Al | Elastic Constant | Value (GPa) |
|-----------|-----|------------------|-------------|
| $\gamma$  | 12  | $C_{11}$         | 270.30      |
|           |     | $C_{12}$         | 149.40      |
|           |     | $C_{44}$         | 112.33      |
| $\gamma'$ | 25  | $C_{11}$         | 211.08      |
|           |     | $C_{12}$         | 164.15      |
|           |     | $C_{44}$         | 125.96      |

from 0 to 0.04 in an interval of 0.01, and energy difference  $E(\delta) - E(0)$  is plotted as a function of  $\delta^2$ . Value of  $C_{44}$  can be obtained by dividing the slope of the line (similar to fig. S1) by the volume  $V$ ,

$$(C_{44}) = \frac{\text{slope of } [E(\delta) - E(0)] \text{ versus } \delta^2}{V}. \quad (7)$$

Calculated values, as reported in Table S1, are in good qualitative agreement with the experimentally reported ones. However, they differ quantitatively from the experimentally reported values by  $\sim 5 - 10\%$  [4]. In this work, phase-field simulations are carried out using values of elastic constants compiled in the comprehensive text published by A. J. Ardell [4].

## 2. Finite Element Analysis of Microstructure

### 2.1. Stress and strain distribution

For doing FEA of microstructure, we need a mesh which is a very good approximation of microstructure morphology. In OOF2, initially, we have a skeleton, which is a grid of elements. This skeleton further gets adapted to the microstructure morphology through skeleton modification tools. From this adapted skeleton, we obtain a mesh that is further solved for stress and strain distribution plots. In this section, we present the adapted skeleton and resulting stress and strain distribution plots for three ageing times at 1000 K for the Ni-Al alloy with an equilibrium  $\gamma'$  volume fraction of 0.4 and 0.6 in figure S2 and S3, and for alloy of equilibrium  $\gamma'$  volume fraction of 0.5 at 900 K and at 1100 K in figure S4 and S5.

### 2.2. Model validation

For validation of our FEM analysis, we study the effect of system size, orientation, applied strain, and mesh size and compare results from two different software packages on our simulated microstructures.

#### 2.2.1. System size

To study the effect of system size we calculate the effective elastic properties for alloy at 1000 K, 0.5  $\gamma'$  equilibrium volume fraction by applying strain of  $3.90625 \times 10^{-2}$  along x-direction for three different system size i.e.  $256 \times 256$ ,  $512 \times 512$  and  $1024 \times 1024$ . There is no significant variation in effective elastic modulus with system size for a specific aging time. Figure S6 shows the effect of system size over effective elastic properties.

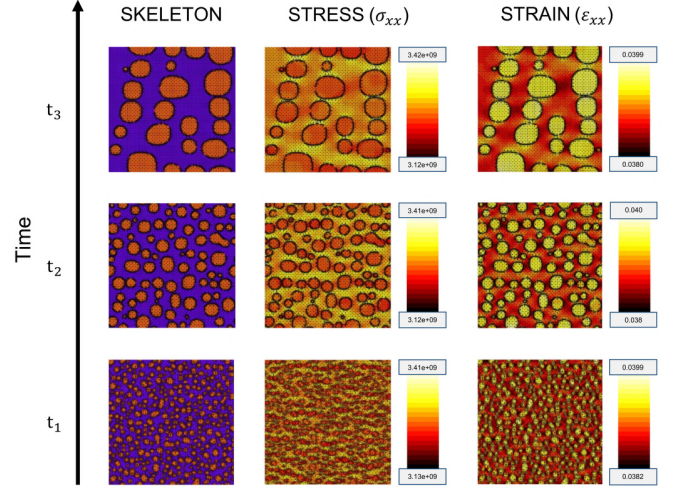

Figure S2: Variation map of simulated microstructures of the Ni-Al alloy along with aging time for equilibrium  $\gamma'$  volume fraction of 0.4 at 1000 K with their respective adapted skeletons and distribution of  $\sigma_{xx}$  and  $\epsilon_{xx}$  obtained after applying uni-axial tensile displacements along the horizontal (or  $x$ ) direction.

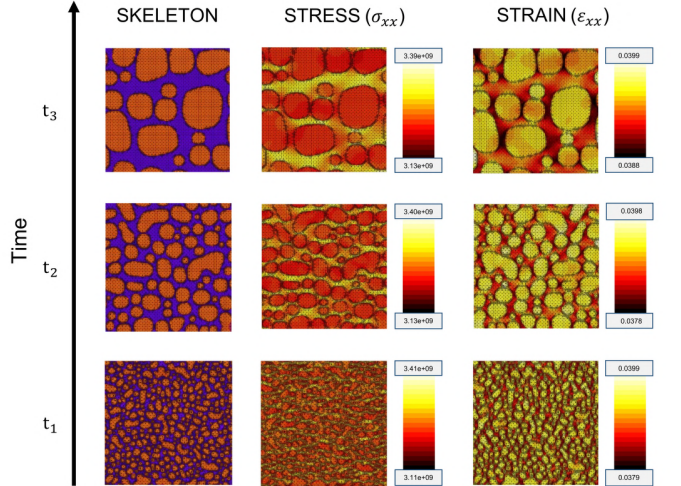

Figure S3: Variation map of simulated microstructures of the Ni-Al alloy along with aging time for equilibrium  $\gamma'$  volume fraction of 0.6 at 1000 K with their respective adapted skeletons and distribution of  $\sigma_{xx}$  and  $\epsilon_{xx}$  obtained after applying uni-axial tensile displacements along the horizontal (or  $x$ ) direction.

#### 2.2.2. Applied strain

We apply three different strains ( $1.953 \times 10^{-4}$ ,  $1.953 \times 10^{-3}$ ,  $1.953 \times 10^{-2}$ ) on the microstructure of the alloy at 1000 K, 0.5  $\gamma'$  equilibrium volume fraction along  $x$ -direction for  $1024 \times 1024$  system size, and calculate its effective elastic properties as shown in Figure S7. The effective elastic properties are constant for different applied strains, so variation of applied strain has no effect on these elastic properties.

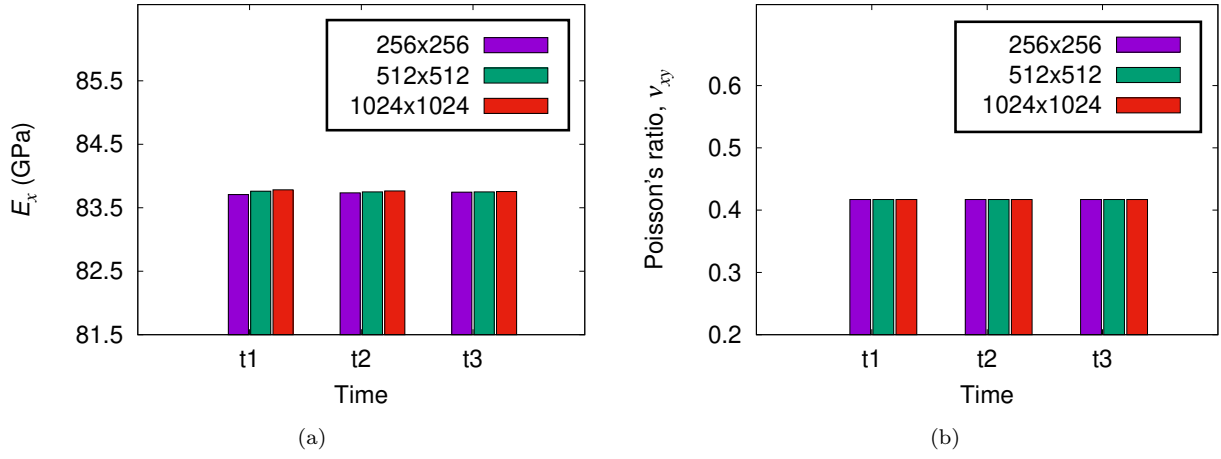

Figure S6: Variation map of effective elastic modulus and effective Poisson's ratio of the alloy along  $x$ -direction at 1000 K with aging time for different system sizes.

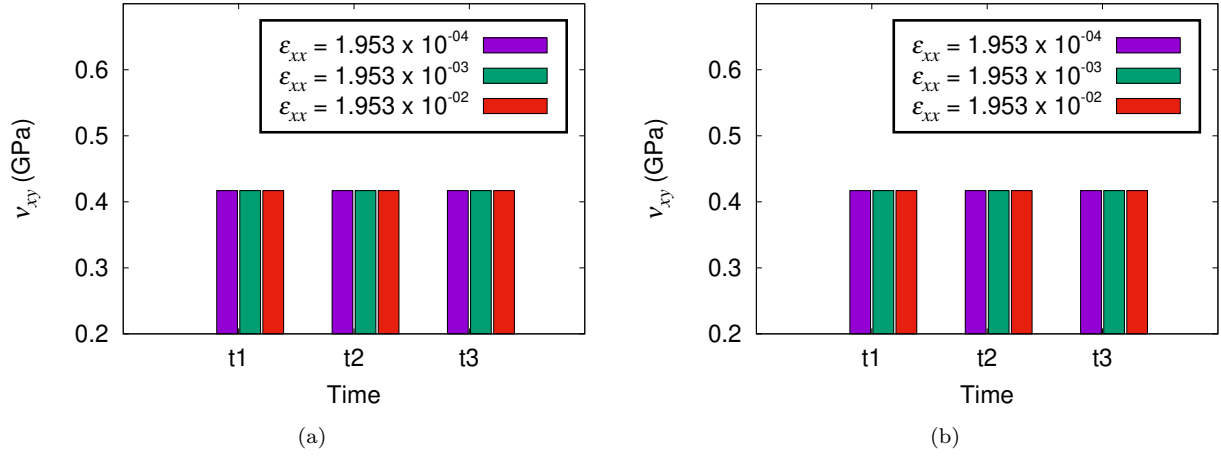

Figure S7: Variation map of effective elastic modulus and effective Poisson's ratio of the alloy along  $x$ -direction at 1000 K, 0.5  $\gamma'$  equilibrium volume fraction with aging time for different applied strain.

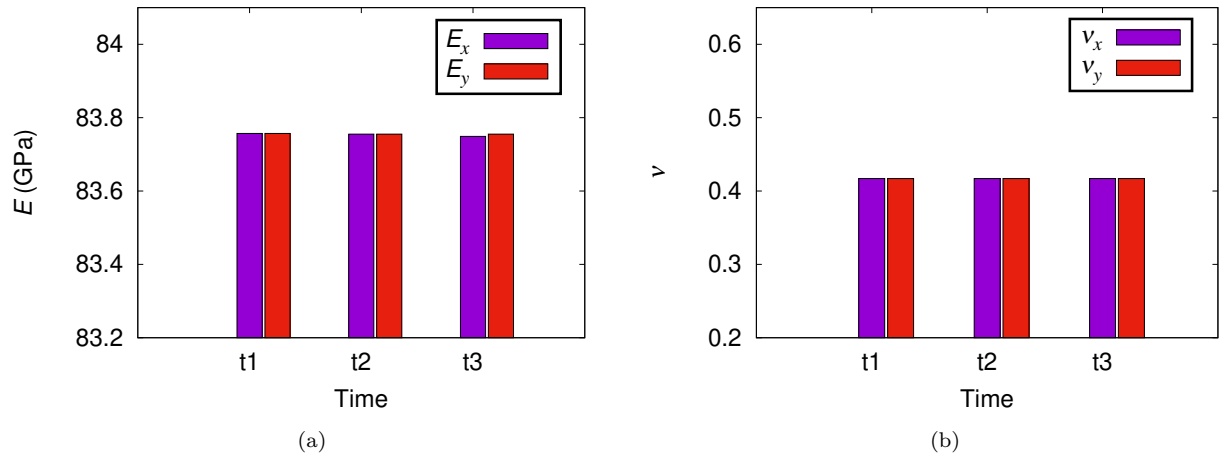

Figure S8: Variation map of effective elastic modulus and Poisson's ratio of the alloy at 1000 K, 0.5  $\gamma'$  equilibrium volume fraction with aging time for different orientation of applied strain.

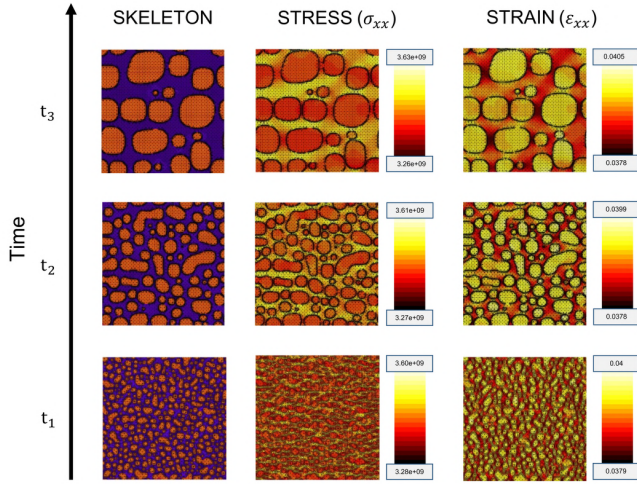

Figure S4: Variation map of simulated microstructures of the Ni-Al alloy along with aging time for equilibrium  $\gamma'$  volume fraction of 0.5 at 900 K with their respective adapted skeletons and distribution of  $\sigma_{xx}$  and  $\epsilon_{xx}$  obtained after applying uni-axial tensile displacements along the horizontal (or  $x$ ) direction.

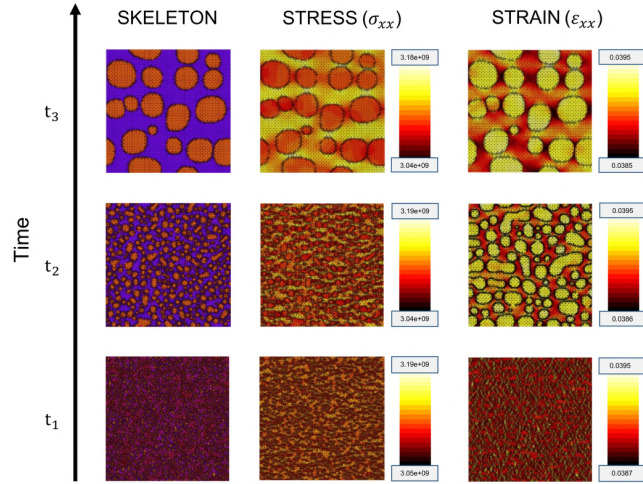

Figure S5: Variation map of simulated microstructures of the Ni-Al alloy along with aging time for equilibrium  $\gamma'$  volume fraction of 0.5 at 1100 K with their respective adapted skeletons and distribution of  $\sigma_{xx}$  and  $\epsilon_{xx}$  obtained after applying uni-axial tensile displacements along the horizontal (or  $x$ ) direction.

### 2.2.3. Orientation of applied strain

We compute the effective elastic properties by applying strain of  $3.90625 \times 10^{-2}$  in two perpendicular directions to the alloy's microstructure at 1000 K, 0.5  $\gamma'$  equilibrium volume fraction for a  $512 \times 512$  system size. As shown in Figure S8, strain orientation with respect to microstructure has no effect on effective elastic modulus and Poisson's ratio.

### 2.2.4. Mesh size

To find the optimum mesh size, we calculate the effective elastic modulus with 5 different initial mesh sizes i.e. 10, 50, 75, 100, and 125. for this study, we take alloy at 1000 K, 0.5  $\gamma'$  equilibrium volume fraction with a system size of  $512 \times 512$  and observe that varying the initial mesh-size didn't have significant impact on the effective elastic properties as shown in figure S9.

### 2.2.5. Result from OOF2 and Abaqus packages

we calculate the effective elastic properties for alloy at 1000 K, 0.4  $\gamma'$  equilibrium volume fraction by applying strain of  $3.90625 \times 10^{-2}$  along  $x$ -direction for three different timestep i.e t<sub>1</sub>, t<sub>2</sub> and t<sub>3</sub>. Results are summarized in Table S2 and S3. Results from both of these software packages are in agreement with each other.

## References

- [1] P. Giannozzi, S. Baroni, N. Bonini, M. Calandra, R. Car, C. Cavazzoni, D. Ceresoli, G.L. Chiarotti, M. Cococcioni, I. Dabo, A. Dal Corso, S. De Gironcoli, S. Fabris, G. Fratesi, R. Gebauer, U. Gerstmann, C. Gougoussis, A. Kokalj, M. Lazzeri, L. Martin-Samos, N. Marzari, F. Mauri, R. Mazarello, S. Paolini, A. Pasquarello, L. Paulatto, C. Sbraccia, S. Scandolo, G. Sclauzero, A.P. Seitsonen, A. Smogunov, P. Umari, and R.M. Wentzcovitch. Quantum espresso: A modular and open-source software project for quantum simulations of materials. *Journal of Physics Condensed Matter*, 21(39), 2009.
- [2] A. Van De Walle, P. Tiwary, M. De Jong, D.L. Olmsted, M. Asta, A. Dick, D. Shin, Y. Wang, L.-Q. Chen, and Z.-K. Liu. Efficient stochastic generation of special quasirandom structures. *Calphad: Computer Coupling of Phase Diagrams and Thermochemistry*, 42:13–18, 2013.
- [3] V. Levitin. *Interatomic Bonding in Solids: Fundamentals, Simulation, and Applications*. Wiley, Hoboken, NJ, 2013.
- [4] A.J. Ardell. The effects of elastic interactions on precipitate microstructural evolution in elastically inhomogeneous nickel-base alloys. *Philosophical Magazine*, 94(19):2101–2130, 2014.

Table S2: Calculated elastic modulus by OOF2 and Abaqus software packages for the alloy with equilibrium 0.4  $\gamma'$  volume fraction at 1000K.

| Timestep | OOF2(GPa) | Abaqus(GPa) |
|----------|-----------|-------------|
| t1       | 84.034    | 84.029      |
| t2       | 84.00     | 84.00       |
| t3       | 83.989    | 83.990      |

Table S3: Calculated Poisson's ratio by OOF2 and Abaqus software packages for alloy with equilibrium 0.4  $\gamma'$  volume fraction at 1000K.

| Timestep | OOF2  | Abaqus |
|----------|-------|--------|
| t1       | 0.417 | 0.417  |
| t2       | 0.417 | 0.417  |
| t3       | 0.417 | 0.417  |

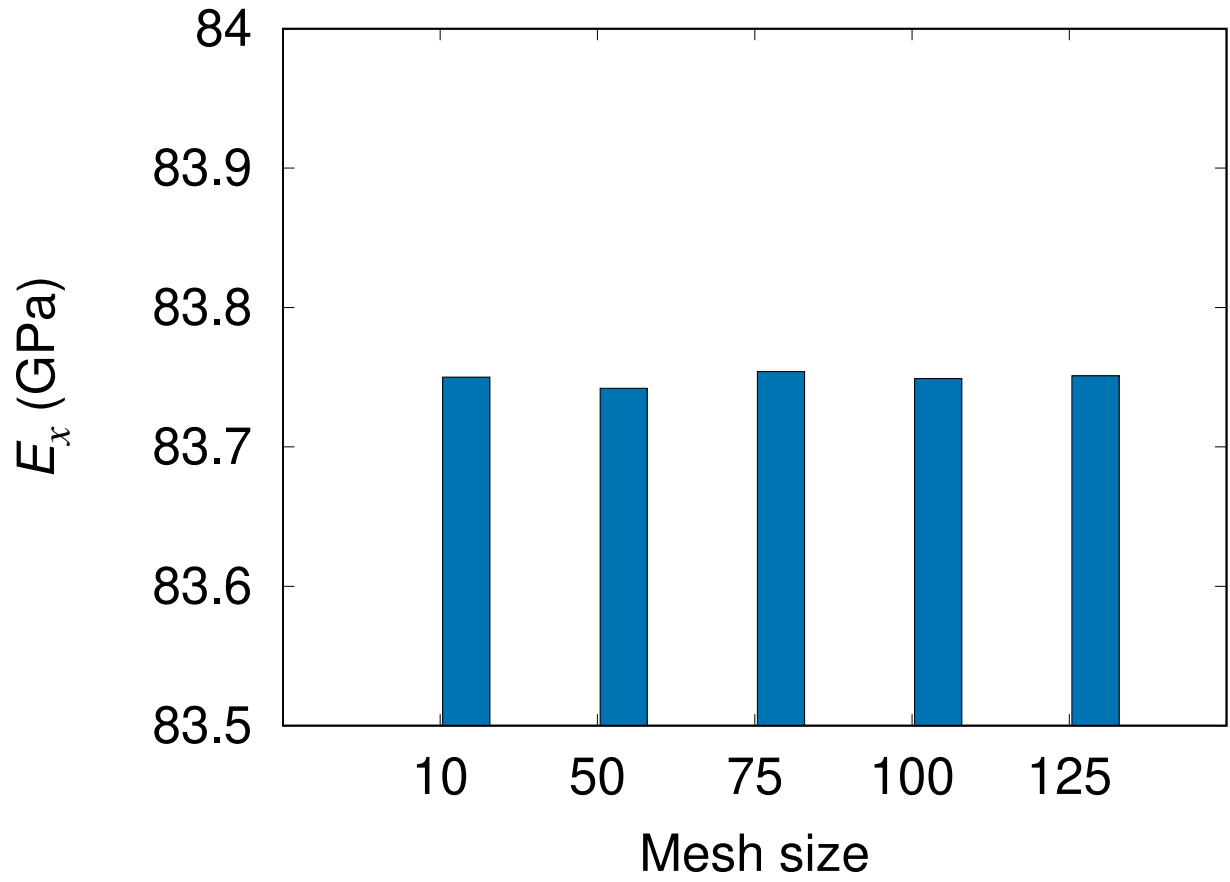

Figure S9: Effect of variation of starting mesh-size on the effective elastic modulus of the alloy along  $x$ -direction at 1000K.

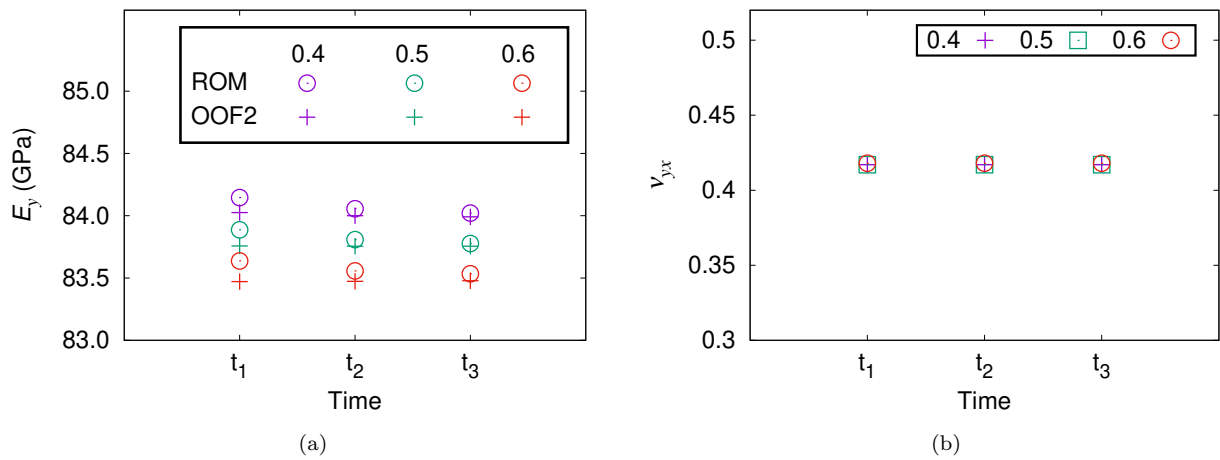

Figure S10: Variation map of effective elastic modulus and poisson's ratio of the alloy along  $y$ -direction with aging times and for three equilibrium  $\gamma'$  volume fractions at 1000 K. Elastic moduli predicted by the rule of mixtures (ROM) are also shown for comparison.

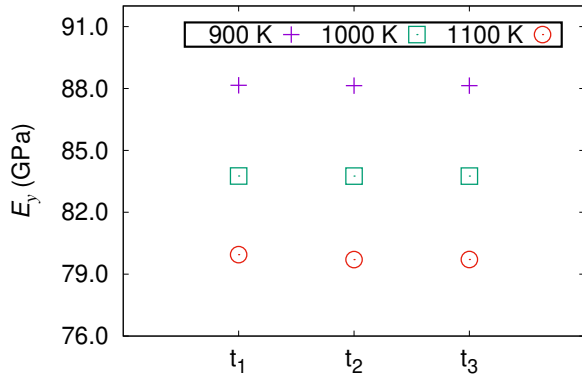

(a)

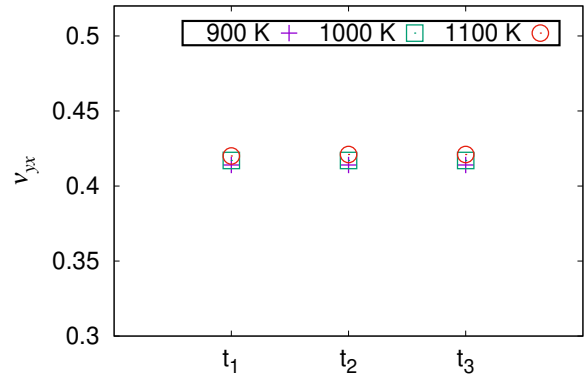

(b)

Figure S11: Variation map of effective elastic modulus and effective Poisson's ratio of the alloy along  $y$ -direction with ageing times at three temperatures for 0.5  $\gamma'$  volume fraction.

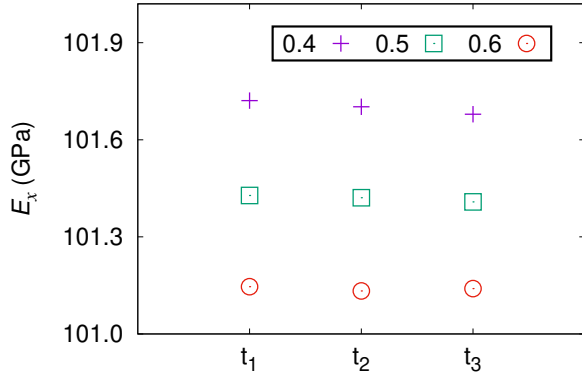

(a)

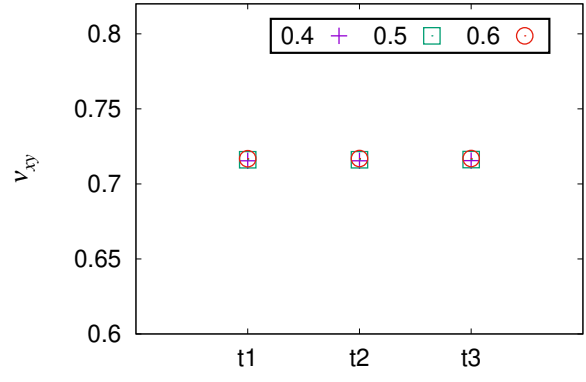

(b)

Figure S12: Variation map of effective elastic modulus and poisson's ratio of the alloy along  $x$ -direction for plane strain condition with aging times and for three equilibrium  $\gamma'$  volume fractions at 1000 K. Elastic moduli predicted by the rule of mixtures (ROM) are also shown for comparison.

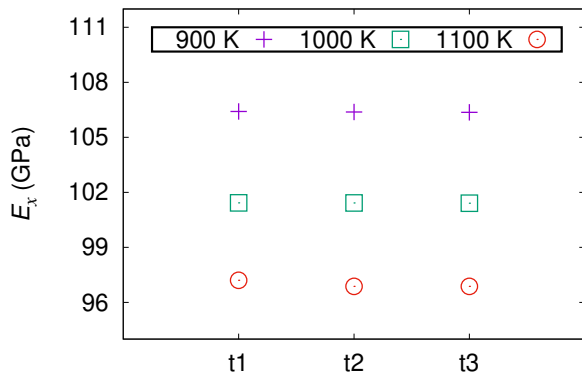

(a)

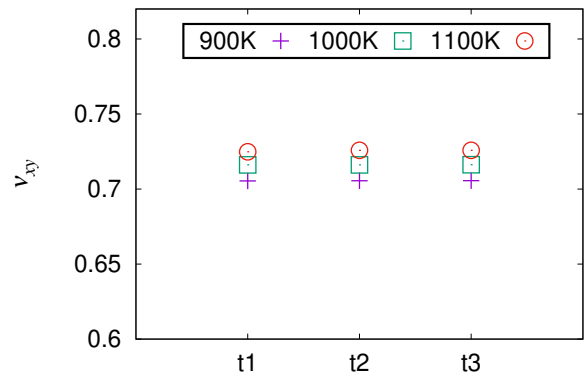

(b)

Figure S13: Variation map of effective elastic modulus and effective Poisson's ratio of the alloy along  $x$ -direction for plane strain condition with aging times at three temperatures for 0.5  $\gamma'$  volume fraction.
